# Supplementary material for: Meta-Learning and Synthetic Data for Automated Pretraining and Finetuning
Source: arXiv:2506.12161 source file (2025-06-11)
Supplement: Supplementary file 1 [file 2022_learningses_soc.pdf]

DocuSign Envelope ID: D077E41F-AD15-43CD-A08A-2772BF136172

**Statement of Contributions for the following publication:**

| | |
|---|---|
| Title | Learning Synthetic Environments and Reward Networks for Reinforcement Learning |
| Link to Publication, DOI | https://iclr.cc/virtual/2022/poster/6495<br>https://openreview.net/forum?id=C1_esHN6AVn |
| Authors | Fabio Ferreira, Thomas Nierhoff, Andreas Sälinger and Frank Hutter |
| Publication Status | Accepted and published |
| Publisher, Date | Proceedings of the 10th International Conference on Learning Representations (ICLR), 2022 |
| Peer-Review-Process | Yes |
| Rank | Ranked A* by the CORE2023 ranking |

**Paper Summary**

This paper introduces a novel approach for training reinforcement learning (RL) agents using synthetic environments (SEs) and reward networks (RNs). These environment models serve as proxies for real environment models that simulate state dynamics and rewards (SEs) or rewards only (RNs) and ultimately allow for a more efficient agent training with fewer interactions than compared to training on the real environments after SE and RN generation. The paper proposes to use a bi-level evolutionary optimization for generating SEs and RNs: the inner loop trains the RL agent and the outer loop trains the parameters of the SE or RN conditional on the performance of the RL agent in the inner loop. The key contributions of the paper are:

1. The paper introduces the novel concept of learning Synthetic Environments and Reward Networks with a bi-level optimization scheme that is guided by the agent performance. The concept allows generating full proxy models that incorporate state dynamics and rewards of real environments that enable training RL agents without any interaction with the actual environments after SE generation.
2. The efficacy of SEs and RNs is demonstrated across several classic control environments such as CartPole, Acrobot (SEs), as well as Cliff Walking, CartPole, MountainCarContinuous, and HalfCheetah (RNs). The study confirms that these proxies can train RL agents effectively while requiring up to 60% fewer training steps.
3. The study shows that these proxies are robust against variations in hyperparameters and capable of transferring learned policies to new, unseen agents, demonstrating their general applicability across different environments and hyperparameter settings.
4. The paper presents empirical evidence showing that SEs and RNs achieve their efficiency gains for training new agents through condensed and informed state and reward representations.

DocuSign Envelope ID: D077E41F-AD15-43CD-A08A-2772BF136172

**Contributions Listing**

| Name | Contributions | Signature |
|---|---|---|
| Fabio Ferreira | Proposed the original idea of Synthetic Environments (SEs) and extending the methodology of Generative Teaching Networks to RL for learning SEs;<br><br>Proposed using the efficiency improvements in training agents on SEs (and Reward Networks (RNs)) and their transferability to other agents as the central novelties of the paper, highlighting a significant gap in the existing related work;<br><br>Co-led the methodology of the project, in particular showed that SEs trained with DDQN agents are able to transfer and generalize to other agents; proposed, implemented, and carried out studies to show that agents require up to 60% fewer training steps when trained on SEs;<br><br>Extended Thomas' code framework by adding baseline agents such as Dueling DDQN, discrete TD3, and improved potential reward shaping functions for RNs, implemented baselines for RNs, e.g., the Intrinsic Curiosity Module (ICM), and together with Thomas, Fabio also worked on hyperparameter optimization and the extension of plotting scripts;<br><br>Owned and was responsible for the code development for assessing efficiency improvements (Fig. 3), gradient flow analysis, and integrating support for running multiple seeds;<br><br>Participated in the periodic code reviews (jointly with Thomas); | DocuSigned by:<br>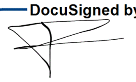<br>CA7363FD31BF45C...<br>15.05.2024 |

| | | |
|---|---|---|
| | Co-carried out approximately 50% of all the experiments (Thomas carried out the other approx. 50%);<br><br>Owned, led and wrote the majority of the paper, including contributions to all parts of the paper. Created the visualizations of the final paper version (except Fig. 2 which was entirely created by Thomas; code for generating Fig. 4 and 5 also was initially created by Thomas and extended by Fabio). Led and contributed significantly to the rebuttal process;<br><br>Created the repository with the final version of the code;<br><br>Supervised Thomas and Andreas. | |
| Thomas Nierhoff | Proposed the idea of using Natural Evolution Strategies (NES) for solving the bi-level optimization necessary to learn synthetic environments and reward networks;<br><br>Discovered the efficiency improvements in training agents on SEs (and Reward Networks (RNs)) and their transferability to other agents.<br><br>Co-led the methodology of the project (showed that SEs trained with DDQN agents are robust towards hyperparameter changes by varying hyperparameters dynamically during training; proposed, implemented, and executed the qualitative studies to shed light on what the agents learn from SEs);<br><br>Co-owned the core implementation, more specifically: implementing the core NES/bi-level optimization framework, the majority of baseline agents (DQN, DDQN, Q-Learning, PPO, SARSA, continuous | DocuSigned by: [signature]<br>04591023C1B749A...<br>16.05.2024 |

DocuSign Envelope ID: D077E41F-AD15-43CD-A08A-2772BF136172

| | | |
|---|---|---|
| | TD3), the whole logic for SE generation (early stopping and evaluation), hyperparameter optimization (jointly with Fabio), parallelization, plotting scripts (jointly with Fabio);<br><br>Co-carried out approximately 50% of all the experiments (Fabio carried out the other approx. 50%);<br><br>Led the periodic code reviews;<br><br>Supported with writing, reviewing and rebutting all parts of the paper but the parts of the paper he had the major contributions were: Related Work (Section 2), Feasibility (Section 5), Analyzing SE Behavior (Section 5), Appendix | |
| Andreas Sälinger | Had a key role in reframing the paper after the prior conference submission (NeurIPS 2021); contributed by clarifying the narrative and enhancing the coherence of the paper;<br><br>Supported with writing, reviewing and rebutting all parts of the paper, but the parts of the paper he had major contributions were: Introduction and Conclusion (both jointly with Fabio);<br><br>Contributed to the rebuttal process (together with Fabio, Thomas and Frank). | DocuSigned by:<br>AADA8541F55A4D6...<br>23/05/2024 |
| Frank Hutter | Helped conceptualize the problem;<br><br>Co-led writing the paper, including contributions to all parts of the paper;<br><br>Helped with reviewing, rebutting and editing the paper;<br><br>Supervised the project and supervised Fabio. | DocuSigned by:<br>Frank Hutter<br>3CDF1E88127C47F...<br>6/28/2024 |
