# Supplementary material for: Meta-Learning and Synthetic Data for Automated Pretraining and Finetuning
Source: arXiv:2506.12161 source file (2025-06-11)
Supplement: Supplementary file 2 [file 2022_onimportance_soc.pdf]

Docusign Envelope ID: 087794CE-A44D-4D5D-AB8F-6237AEAFA85B

**Statement of Contributions for the following publication:**

| | |
|---|---|
| Title | On the Importance of Hyperparameters and Data Augmentation for Self-Supervised Learning |
| Link to Publication, DOI | https://arxiv.org/pdf/2207.07875<br>https://openreview.net/forum?id=oBmAN382UL |
| Authors | Diane Wagner, Fabio Ferreira, Danny Stoll, Robin Tibor Schirrmeister, Samuel Müller, Frank Hutter |
| Publication Status | Accepted at the First Workshop of Pre-training: Perspectives, Pitfalls, and Paths Forward at ICML 2022 |
| Publisher, Date | - |
| Peer-Review-Process | Yes |
| Rank | not ranked by CORE2023 (workshop) |

**Paper Summary**

This paper investigates the influence of hyperparameters and data augmentation strategies on Self-Supervised Learning (SSL), using SimSiam with a ResNet-18 backbone across CIFAR-10, CIFAR-100, and DermaMNIST datasets. The study focuses on understanding the role of data augmentation in SSL, examining whether better augmentation strategies can significantly improve performance. It also explores which hyperparameters are most likely to cause model collapse when set incorrectly, and which hyperparameters should be prioritized to achieve high performance and outperform baselines in SSL.

The results reveal that while hyperparameter optimization provides marginal improvements, data augmentation has a far more substantial impact on SSL performance. As an additional contribution, the authors introduce GroupAugment, a novel automated data augmentation algorithm that optimizes sampling across groups of augmentations. GroupAugment consistently delivers superior accuracy in linear evaluation protocols across all datasets, outperforming existing augmentation techniques.

Additionally, the paper presents a detailed empirical analysis, offering insights into the importance of hyperparameter tuning and its effects on model stability and performance. This work highlights the often-underestimated role of data augmentation in SSL and provides practical insights for optimizing SSL pipelines through improved augmentation strategies. The key contributions of the paper are:

1. The paper investigates the role of hyperparameters and data augmentation in Self-Supervised Learning (SSL), identifying key factors that influence performance, including potential causes of model collapse.
2. The paper proposes GroupAugment, a novel automated data augmentation algorithm that optimizes sampling across groups of augmentations. It outperforms existing data augmentation strategies used in Supervised and Self-Supervised Learning across multiple datasets.

Docusign Envelope ID: 087794CE-A44D-4D5D-AB8F-6237AEAFA85B

3. The paper provides insights into which hyperparameters are critical to optimize for achieving high SSL performance and avoiding model collapse.

**Contributions Listing**

| **Name** | **Contributions** | **Signature** |
|---|---|---|
| Diane Wagner | Proposed the idea to investigate hyperparameter and data augmentation in SSL, highlighting their key role in downstream task performance (jointly with Fabio)<br><br>Owned and led all code implementations required for the paper;<br><br>Owned, led, and carried out all experiments and created all figures and tables in the paper;<br><br>Co-led the methodology of the project jointly with Fabio;<br><br>Proposed, developed, evaluated, and analyzed GroupAugment (jointly with Danny);<br><br>Contributed to shaping the project's vision and methodology in collaboration with the supervisory team.<br><br>Lead the periodic code reviews;<br><br>Co-wrote the paper and positioned the work in the research context together with Fabio and Danny. | Signiert von:<br>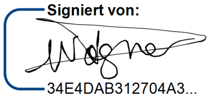<br>34E4DAB312704A3...<br>31.10.2024 |

Docusign Envelope ID: 087794CE-A44D-4D5D-AB8F-6237AEAFA85B

| | | |
|---|---|---|
| Fabio Ferreira | Proposed the idea to investigate hyperparameter and data augmentation in SSL, highlighting their key role in downstream task performance (jointly with Diane)<br><br>Guided the project direction and co-led the methodology of the project jointly with Diane;<br><br>Provided the initial code for training ResNet-18 with SimSiam, as well as the code for linear evaluation and support for CIFAR-10 and CIFAR-100;<br><br>Co-designed the experimental setup jointly with Diane and Danny;<br><br>Participated in the periodic code reviews (jointly with Diane);<br><br>Contributed to shaping the project's vision and methodology in collaboration with the supervisory team.<br><br>Owned and lead the paper writing, co-wrote the paper and positioned the work in the research context together with Diane and Danny.<br><br>Lead the supervision of Diane. | DocuSigned by:<br>CA7363FD31BF45C...<br>28.10.2024 |
| Danny Stoll | Co-supervised the project alongside Fabio, Robin, and Samuel;<br><br>Contributed to shaping the project's vision and methodology;<br><br>Proposed, developed, evaluated, and analyzed GroupAugment (jointly with Diane);<br><br>Co-designed the experimental setup jointly with Diane and Fabio; | Signed by:<br>D2A3985244F3484...<br>04/11/2024 |

Docusign Envelope ID: 087794CE-A44D-4D5D-AB8F-6237AEAFA85B

| | | |
|---|---|---|
| | Co-wrote the paper and positioned the work in the research context with Diane and Fabio and contributed by clarifying the narrative and enhancing the coherence of the paper. | |
| Robin Tibor Schirrmeister | Co-supervised the project alongside Fabio, Danny, and Samuel;<br><br>Offered insights on related work and helped refine the narrative within the broader context of medical machine learning;<br><br>Assisted in writing the paper, particularly the introduction section;<br><br>Supported with reviewing all parts of the paper. | Signed by:<br>9C5A138D83524AE...<br>10/28/2024 |
| Samuel Müller | Co-supervised the project alongside Fabio, Danny, and Robin;<br><br>Contributed to the initial code development and early experimental design, providing foundational assistance for the project;<br><br>Supported with reviewing all parts of the paper. | Signed by:<br>Samuel Müller<br>D963AEAD51FC4C0...<br>10/29/2024 |
| Frank Hutter | Helped conceptualize the problem;<br><br>Supported in writing, reviewing, and editing the paper;<br><br>Supervised the project and supervised Fabio, Danny, Robin, Samuel. | Signed by:<br>3CDF1E88127C47F...<br>31/10/2024 |
