# Supplementary material for: Meta-Learning and Synthetic Data for Automated Pretraining and Finetuning
Source: arXiv:2506.12161 source file (2025-06-11)
Supplement: Supplementary file 3 [file 2022_zap_soc.pdf]

DocuSign Envelope ID: EBFACF60-0B79-4D40-ACD8-96907C241CB3

**Statement of Contributions for the following publication:**

| | |
|---|---|
| Title | Zero-shot AutoML with Pretrained Models |
| Link to Publication, DOI | https://proceedings.mlr.press/v162/ozturk22a |
| Authors | Ekrem Öztürk*, Fabio Ferreira*, Hadi Jomaa*, Lars Schmidt-Thieme, Josif Grabocka and Frank Hutter (*: joint first author) |
| Publication Status | Accepted and published |
| Publisher, Date | Proceedings of the 39th International Conference on Machine Learning (ICML), 2022 |
| Peer-Review-Process | Yes |
| Rank | Ranked A* by the CORE2023 ranking |

**Paper Summary**

The paper "Zero-Shot AutoML with Pretrained Models" introduces an innovative approach to Automated Machine Learning (AutoML) that leverages pretrained models and meta-learning to select and tune deep learning pipelines without requiring any exploratory evaluations on new datasets. It enables efficient model and hyperparameter selection under resource constraints and contributes to the fields of meta-learning and AutoML. The key contributions of the paper are:

1. The study extends traditional automated machine learning approaches by using meta-learning to learn a selector that chooses the right pretrained model and finetuning hyperparameters (referred to as a “deep learning pipeline”) for unseen image classification datasets conditioned only on the dataset meta-features (“zero-shot”).
2. The paper provides a large-scale meta-dataset comprising evaluations of 525 deep learning pipelines across 525 popular image classification datasets. This dataset is used for meta-learning the selector and is one of the largest of its kind at the time of the paper publication.
3. The paper introduces a novel methodology for zero-shot AutoML, beginning with the development of a powerful meta-selector known as “ZAP-AS”. This meta-selector leverages the algorithm selection system “AutoFolio”, which incorporates techniques from regression, classification, clustering, and cost-sensitive classification. ZAP-AS operates independently of geometric spaces, focusing instead on algorithmic selection without exploiting correlated spatial information about deep learning pipelines. Subsequently, the paper presents “ZAP-HPO”, which approaches the pipeline selection by formulating it as an algorithm selection problem within a geometric space. In contrast to ZAP-AS, this method utilizes a ranking objective for pipelines.
4. The proposed approach was evaluated in the ChaLearn AutoDL challenge under tight computational constraints and demonstrated superior performance, significantly outperforming all competition entries and baselines.

DocuSign Envelope ID: EBFACF60-0B79-4D40-ACD8-96907C241CB3

**Contributions Listing**

| **Name** | **Contributions** | **Signature** |
|---|---|---|
| Fabio Ferreira | As the core developer and main contributor of the AutoML Freiburg Lab's submission to the AutoDL challenge 2019 [1], Fabio laid the foundation of the project by providing all project code to Ekrem, who extended and scaled up the idea to more datasets, better augmentation methods and tuned ZAP-AS models. The code from Fabio included the meta-dataset collection/curation, meta-dataset augmentation, Hyperparameter Optimization (HPO) scripts for generating the meta-dataset, training logic for ZAP-AS with AutoFolio, cluster submissions and experiment execution;<br><br>Supported Ekrem on the code-level through code reviews and small code changes (e.g., meta-dataset augmentation).<br><br>Proposed and defined the DL pipeline hyperparameter search space (jointly with Frank), as well as the meta-dataset design including the meta-dataset augmentations present in the paper;<br><br>Co-led the project's methodology and overall strategic direction (jointly with Frank);<br><br>Ran initial ZAP-AS model experiments and tuned its early versions on a smaller version of the meta-dataset for the challenge submission; analyzed the effect of simple and complex meta-features on the performance of ZAP-AS; the analysis of how simple and complex meta-features impact the performance of ZAP-AS/ZAP-HPO was incorporated into the final evaluations and conclusions presented in the paper; | DocuSigned by:<br>CA7363FD31BF45C...<br>29.05.2024 |

| | | |
|---|---|---|
| | Owned, led and wrote the majority of the paper, including contributions to all parts of the paper and creating figures 1 and 2; led and contributed significantly to the rebuttal process;<br><br>Supervised Ekrem Öztürk.<br><br>[1] Zhengying Liu, Adrien Pavao, Zhen Xu, Sergio Escalera, Fabio Ferreira, et al., *Winning solutions and post-challenge analyses of the chalearn autodl challenge 2019*. IEEE Transactions on Pattern Analysis and Machine Intelligence, 43(9):3108–3125, 2021. | |
| Ekrem Öztürk | Owned and led the extension of the AutoDL competition code from Fabio, which included adding more datasets to the meta-dataset, running the HPO with larger budgets for the DL pipelines that resulted in the large-scale meta-dataset (present in paper), finetuned the ZAP-AS models, and implemented all baseline methods;<br><br>Executed all ZAP-AS meta-trainings on the extended meta-dataset and some ZAP-HPO experiments for the rebuttal;<br><br>Supported with writing, editing, reviewing and rebutting all parts of the paper, but the parts of the paper he had the major contributions were: ZAP Meta-Dataset Design (Section 4), Experiments (Section 5), and Figures 4-6. | DocuSigned by:<br>Ekrem Öztürk<br>183B3C77C1A24B6...<br>30/05/2024 |

| | | |
|---|---|---|
| Hadi Jomaa | Owned and led the implementation and training of ZAP-HPO, including defining its hyperparameter configuration space;<br><br>Ran the ZAP-HPO experiments for the initial paper submission (Ekrem executed the experiments for the rebuttal);<br><br>Supported with writing, editing, and reviewing all parts of the paper, but the parts of the paper he had the major contributions were: Related Work (Section 2), ZAP via Zero-Shot HPO (ZAP-HPO) (Section 3.3), Experiments (Section 5), and Figure 3. | DocuSigned by:<br>Hadi Samer Jomaa<br>1503474931CA43A...<br>30.05.2024 |
| Lars Schmidt-Thieme | Helped with reviewing, rebutting and editing the paper;<br><br>Supervision of Hadi Jomaa. | DocuSigned by:<br>Lars Schmidt-Thieme<br>4E66175AA1DF4F1...<br>6/7/2024 |
| Josif Grabocka | Proposed the idea of using a ranking surrogate objective;<br><br>Helped conceptualize the problem;<br><br>Co-led writing the paper, including contributions to all parts of the paper;<br><br>Helped with reviewing, rebutting and editing the paper. | DocuSigned by:<br>Josif Grabocka<br>257E43784D71473...<br>6/8/2024 |
| Frank Hutter | Proposed the original idea for tackling the problem specification of the AutoDL challenge with a meta-learned algorithm selection surrogate model based on deep learning pipeline meta-training data;<br><br>Helped conceptualize the problem;<br><br>Co-led writing the paper, including contributions to all parts of the paper; | DocuSigned by:<br>Frank Hutter<br>3CDF1E88127C47F...<br>6/28/2024 |

| | | |
|---|---|---|
| | Helped with reviewing, rebutting and editing the paper.<br><br>Supervised the project and Fabio Ferreira. | |
