# Supplementary material for: Meta-Learning and Synthetic Data for Automated Pretraining and Finetuning
Source: arXiv:2506.12161 source file (2025-06-11)
Supplement: Supplementary file 4 [file 2024_hvp_soc.pdf]

Docusign Envelope ID: 2F7288D1-2DDE-46C8-A08F-41A0064DF9F9

**Statement of Contributions for the following publication:**

| | |
|---|---|
| Title | Beyond Random Augmentations: Pretraining with Hard Views |
| Link to Publication, DOI | https://arxiv.org/abs/2310.03940<br>https://openreview.net/forum?id=AK1C55o4r7 |
| Authors | Fabio Ferreira*, Ivo Rapant*, Jörg Franke, and Frank Hutter<br>(*: joint first author) |
| Publication Status | Accepted and published |
| Publisher, Date | Proceedings of the Thirteenth International Conference on Learning Representations (ICLR), 2025 |
| Peer-Review-Process | Yes |
| Rank | Ranked A* by the CORE2023 ranking |

**Paper Summary**

Many Self-Supervised Learning (SSL) methods aim for a model invariance to different image augmentations known as *views*. The paper "Beyond Random Augmentations: Pretraining with Hard Views" introduces Hard View Pretraining (HVP), an approach to Self-Supervised Learning (SSL) that extends the conventional random view sampling by explicitly selecting views that benefit the learning process. By exposing the model to harder, more challenging samples during SSL pretraining, the model achieves higher downstream task performance. The key contributions of the paper are:

1. Proposing to use HVP that automatically exposes the model to harder samples (views) during pretraining. It only requires the computability of sample-wise losses and is easily integrated into existing SSL pipelines.
2. The study demonstrates the effectiveness and compatibility using ImageNet-1k across four popular SSL methods (DINO, iBOT, SimSiam, SimCLR), achieving linear evaluation accuracy improvements of 1% on average.
3. The paper shows that HVP-pretrained models also yield performance improvements on a diverse set of transfer tasks, including finetuning, object detection, and segmentation.
4. The study also presents insights into the underlying mechanisms and robustness of HVP.

Docusign Envelope ID: 2F7288D1-2DDE-46C8-A08F-41A0064DF9F9

**Contributions Listing**

| Name | Contributions | Signature |
|---|---|---|
| Fabio Ferreira | Proposed the original idea of adversarially learning a view network to output hard views to challenge a model during SSL pretraining. Fabio implemented an initial version of this idea with DINO and SimSiam. Ivo investigated and enhanced this idea further in the scope of his student project that Fabio supervised. Ultimately, the idea was dismissed due to computational instability. To understand the adversary network's behavior better, Ivo proposed forwarding multiple randomly sampled views and selecting those with the highest loss for the backward pass, which improved downstream task performance. Fabio encouraged further development of this method in Ivo's master thesis for other SSL methods and transfer tasks, leading to the present paper;<br><br>Provided base code for training DINO and SimSiam on ImageNet on the cluster infrastructure; implemented transfer tasks for linear evaluation and finetuning (Table 2) and baselines (BarlowTwins; not in the paper); proposed and investigated methods to make HVP more efficient (jointly with Ivo)<br><br>Owned and led the project's methodology and overall strategic direction, including the methods used in the empirical analysis Section;<br><br>Co-carried out approximately 50% of all the experiments (Ivo carried out the other approx. 50%);<br><br>Owned, led and wrote the majority of the paper, including contributions to all parts of the paper; led and contributed significantly to the rebuttal process; | DocuSigned by:<br>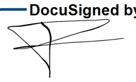<br>CA7363FD31BF45C...<br>22.01.2025 |

Docusign Envelope ID: 2F7288D1-2DDE-46C8-A08F-41A0064DF9F9

| | | |
|---|---|---|
| | Supported Ivo on the code-level through code reviews and small code changes.<br><br>Supervised Ivo Rapant. | |
| Ivo Rapant | Proposed the idea of forwarding multiple random views and selecting the hardest for the backward pass;<br><br>Developed further the DINO and SimSiam base code from Fabio; implemented HVP, implemented baselines (iBOT, SimCLR), proposed and investigated methods to make HVP more efficient (jointly with Fabio);<br><br>Carried out the empirical analysis of HVP, as well as the object detection and instance segmentation transfer task experiments;<br><br>Co-carried out approximately 50% of all the experiments (Fabio carried out the other approx. 50%);<br><br>Supported with writing, editing, reviewing and rebutting all parts of the paper, but the parts of the paper he had the major contributions were: Main Results (Section 4), Empirical Analysis (Section 5) | Signed by:<br>E18D86EC0C94416...<br>1/23/2025 |

Docusign Envelope ID: 2F7288D1-2DDE-46C8-A08F-41A0064DF9F9

| | | |
|---|---|---|
| Jörg Franke | Supported in reframing the paper; contributed by clarifying the narrative and enhancing the coherence of the paper;<br><br>Supported with writing and reviewing all parts of the paper, but the parts of the paper he had major contributions were: Introduction and Conclusion (both jointly with Fabio);<br><br>Supported in running long-run experiments on one of the Juwels clusters. | Signed by:<br>Jörg Franke<br>DC6598DF2302491...<br>1/24/2025 |
| Frank Hutter | Helped conceptualize the problem;<br><br>Co-led writing the paper, including contributions to all parts of the paper;<br><br>Helped with reviewing, rebutting and editing the paper;<br><br>Supervised the project and supervised Fabio Ferreira. | Signed by:<br>Frank Hutter<br>3CDF1E88127C47F...<br>1/22/2025 |
