# Supplementary material for: Meta-Learning and Synthetic Data for Automated Pretraining and Finetuning
Source: arXiv:2506.12161 source file (2025-06-11)
Supplement: Supplementary file 5 [file 2024_oswm_soc.pdf]

Docusign Envelope ID: BD53F80E-F102-420E-9204-4C202DCB334D

**Statement of Contributions for the following publication:**

| | |
|---|---|
| Title | One-shot World Models Using a Transformer Trained on a Synthetic Prior |
| Link to Publication, DOI | https://arxiv.org/abs/2409.14084 |
| Authors | Fabio Ferreira*, Moreno Schlageter*, Raghu Rajan, André Biedenkapp and Frank Hutter (*: joint first author) |
| Publication Status | Accepted at the NeurIPS 2024 Workshop on Open-World Agents |
| Publisher, Date | - |
| Peer-Review-Process | Yes |
| Rank | not ranked by CORE2023 (workshop) |

**Paper Summary**

This paper introduces One-Shot World Models (OSWM), a novel transformer-based approach for building world models entirely from synthetic data. OSWM is trained using a synthetic prior composed of randomly initialized and untrained neural networks, which simulate the state dynamics and reward functions of target environments. By leveraging in-context learning, the model adapts to new environments with minimal real-world interactions. Specifically, OSWM can rapidly adapt using only 1,000 sampled transition steps as context, allowing it to train agents for various simple reinforcement learning tasks. The method has been shown to solve tasks in environments such as GridWorld, CartPole, and a custom control environment, demonstrating its effectiveness in learning policies for different simple environments. However, performance was less consistent in the more complex Reacher environment, where the model achieved only mediocre results. Despite this, the use of synthetic priors to generate diverse environment dynamics presents a promising direction for efficient world model training without needing extensive real-world data. The key contributions of the paper are:

1. Introduction of OSWM, a transformer-based world model trained on synthetic data from a prior of randomly initialized and untrained neural networks simulating environment dynamics and rewards.
2. Rapid Adaptation via In-Context Learning: After training on synthetic prior data, OSWM adapts to new environments and serves as a proxy using only 1,000 sampled interaction steps from the target environment during inference.
3. The paper shows that OSWM effectively trains agents for GridWorld, CartPole, and a custom control environment.
4. The paper provides an empirical analysis that assesses the importance of context sampling and include an ablation study on the design of the synthetic prior.

Docusign Envelope ID: BD53F80E-F102-420E-9204-4C202DCB334D

**Contributions Listing**

| Name | Contributions | Signature |
|---|---|---|
| Fabio Ferreira | Proposed the original idea of One-Shot World Models (OSWM) using synthetic priors;<br><br>Developed the overall methodology of the project and guided its direction;<br><br>Owned, led, and wrote the majority of paper and created Figure 1;<br><br>Provided critical insights for positioning the paper within the context of related work and framed the key contributions;<br><br>Lead the supervision of Moreno. | DocuSigned by:<br>CA7363FD31BF45C...<br>28.10.2024 |
| Moreno Schlageter | Owned and led the implementation and experimentation for OSWM and developed the code for training OSWM;<br><br>Ran all experiments and created the majority of figures (excluding Figure 1);<br><br>Proposed the logic for the NN and Momentum prior, worked on the core OSWM architecture and implemented the synthetic prior mechanism;<br><br>Led and executed all experimental evaluations across various environments, including all experiments on sampling context, as well as on analyzing and ablating the prior;<br><br>Contributed to shaping the project's vision and methodology in collaboration with the supervisory team;<br><br>Supported with writing and reviewing all parts of the paper. | Signiert von:<br>Moreno Schlageter<br>6E9AEF629B124B3...<br>28.10.2024 |

| | | |
|---|---|---|
| Raghu Rajan | Co-supervised the project alongside Fabio and André;<br><br>Contributed to shaping the project's vision and methodology;<br><br>Supported in framing and writing of the paper, contributed by clarifying the narrative and enhancing the coherence of the paper;<br><br>Offered insights on related work and helped refine the narrative within the broader context of reinforcement learning research. | DocuSigned by:<br>D7AAC25D7CCF49D...<br>10/28/2024 |
| André Biedenkapp | Co-supervised the project alongside Fabio and Raghu;<br><br>Contributed to shaping the project's vision and methodology;<br><br>Supported in framing and writing of the paper, contributed by clarifying the narrative and enhancing the coherence of the paper;<br><br>Offered insights on related work and helped refine the narrative within the broader context of reinforcement learning research. | DocuSigned by:<br>B57C612393B6408...<br>10/28/2024 |
| Frank Hutter | Helped conceptualize the problem;<br><br>Supported in reviewing, and editing the paper;<br><br>Supervised the project and supervised Fabio, Raghu, and André. | Signed by:<br>3CDF1E88127C47F...<br>31/10/2024 |
