# Supplementary material for: Meta-Learning and Synthetic Data for Automated Pretraining and Finetuning
Source: arXiv:2506.12161 source file (2025-06-11)
Supplement: Supplementary file 6 [file 2024_qtt_soc.pdf]

Docusign Envelope ID: AE5870B0-C1EA-4BDB-921C-224680F57BC3

**Statement of Contributions for the following publication:**

| | |
|---|---|
| Title | Quick-Tune-Tool: A Practical Tool and its User Guide for Automatically Finetuning Pretrained Models |
| Link to Publication, DOI | https://openreview.net/forum?id=d0Hapti3Uc |
| Authors | Ivo Rapant, Lennart Purucker, Fabio Ferreira, Sebastian Pineda Arango, Arlind Kadra, Josif Grabocka, and Frank Hutter |
| Publication Status | Accepted at the AutoML Conference 2024 (Workshop Track) |
| Publisher, Date | Proceedings of the third International Conference on Automated Machine Learning (AutoML), 2024 |
| Peer-Review-Process | Yes |
| Rank | not ranked by CORE2023 |

**Paper Summary**

This paper introduces Quick-Tune-Tool, a tool that simplifies the selection and finetuning of pretrained models, with a focus on image classification tasks. The tool is built on the QuickTune algorithm [1], which abstracts research-level code into an accessible, user-friendly interface designed for machine learning practitioners. Given the growing complexity and variety of pretrained models available, Quick-Tune-Tool aims to help users determine the most suitable pretrained model and optimize its finetuning strategy without extensive trial-and-error.

The contributions of this paper include the release of Quick-Tune-Tool, offering a detailed architectural overview of its design, a user guide for image classification, and empirical evaluations. It was evaluated on four commonly used image classification datasets: Oxford Flowers 102, Stanford Cars, Imagenette, and FGVC-Aircraft. The experiments demonstrate that Quick-Tune-Tool not only simplifies the finetuning process, but also consistently outperforms random search baselines in terms of top-1 accuracy and speed of convergence.

With its straightforward adaptability, Quick-Tune-Tool is positioned as a practical solution for automating finetuning workflows, providing significant value to practitioners working on image classification tasks. The tool's architecture has been designed with future adaptability in mind, allowing for off-the-shelf adaptation to other domains. The key contributions of the paper are:

1. The paper introduces *Quick-Tune-Tool*, which abstracts the QuickTune algorithm [1] into a user-friendly tool designed to automate model selection and finetuning for image classification tasks.
2. It provides a detailed architectural overview of *Quick-Tune-Tool*, explaining its components and functionality, alongside a comprehensive user guide that enables users to implement the tool with just a few lines of code. It allows easy adaptation to other domains.
3. The authors conduct empirical evaluations on four widely-used image classification datasets – Oxford Flowers 102, Stanford Cars, Imagenette, and FGVC-Aircraft,

Docusign Envelope ID: AE5870B0-C1EA-4BDB-921C-224680F57BC3

demonstrating the tool’s effectiveness in outperforming random search in both accuracy and convergence speed.

[1] Arango, S. P., Ferreira, F., Kadra, A., Hutter, F., & Grabocka, J. (2024). *Quick-Tune: Quickly Learning Which Pretrained Model to Finetune and How*. In The Twelfth International Conference on Learning Representations (ICLR 2024). Paper: https://openreview.net/forum?id=tqh1zdXIra

**Contributions Listing**

| **Name** | **Contributions** | **Signature** |
|---|---|---|
| Ivo Rapant | Owned and led the development of *Quick-Tune-Tool* and handled all core implementations;<br><br>Owned, led, and implemented all experiments conducted;<br><br>Contributed to shaping the project's vision and methodology in collaboration with the supervisory team;<br><br>Owned and led the writing of the paper, as well as reviewing and rebutting it. | Signed by:<br>E18D86EC0C94416...<br>10/22/2024 |
| Lennart Purucker | Co-supervised the project alongside Fabio;<br><br>Contributed to shaping the project's vision and methodology in collaboration with the supervisory team;<br><br>Contributed substantially to writing, reviewing, and rebutting the paper, including positioning it within the broader research context;<br><br>Helped design the API and provided input on the use cases of the tool;<br><br>Co-led supervision during the later phases of the project. | Signiert von:<br>Lennart Oswald Purucker<br>6A52A22B8876416...<br>22.10.2024 |

Docusign Envelope ID: AE5870B0-C1EA-4BDB-921C-224680F57BC3

| | | |
|---|---|---|
| Fabio Ferreira | Initiated the project with Frank and supervised Ivo in the first third of the project; later co-supervised with Lennart;<br><br>Contributed to defining the API and tool use cases (initially with Ivo, then jointly with Lennart);<br><br>Provided input on shaping the vision of the tool;<br><br>Supported in writing the paper and addressed questions related to the DINOv2 experiments.<br><br>Contributed to shaping the project's vision and methodology;<br><br>Helped in writing, reviewing, and rebutting the paper. | DocuSigned by:<br>CA7363FD31BF45C...<br>22.10.2024 |
| Sebastian Pineda Arango | Co-supervised the project alongside Lennart and Fabio;<br><br>Supported Ivo with the original QuickTune code (of which Sebastian is the core author) and debugging the method;<br><br>Contributed to steering the project;<br><br>Helped in writing, reviewing, and rebutting the paper; provided input on related work; | DocuSigned by:<br>Sebastian Pineda Arango<br>FC1C0379C4234BB...<br>10/23/2024 |
| Arlind Kadra | Helped steer the project and provided advice on baselines;<br><br>Helped in writing, reviewing, and rebutting the paper. | DocuSigned by:<br>655FFB067F26476...<br>10/24/2024 |

| | | |
|---|---|---|
| Josif Grabocka | Helped in writing, reviewing, and rebutting the paper;<br><br>Supervised Sebastian and Arlind. | Signed by:<br>257E43784D71473...<br>10/24/2024 |
| Frank Hutter | Proposed the initial idea to develop a tool based on the QuickTune paper [1];<br><br>Proposed the tool's adaptation to domains like image segmentation or large language models; and overall contributed to shaping the project's vision and methodology;<br><br>Helped in writing, reviewing, and rebutting the paper;<br><br>Supervised the project and supervised Ivo, Lennart, and Fabio. | Signed by:<br>3CDF1E88127C47F...<br>25/10/2024 |
