# Supplementary material for: Meta-Learning and Synthetic Data for Automated Pretraining and Finetuning
Source: arXiv:2506.12161 source file (2025-06-11)
Supplement: Supplementary file 7 [file 2024_quicktune_llms.pdf]

Docusign Envelope ID: 5105FC86-E829-4EE8-A6B6-9CAA69FF6C4B

**Statement of Contributions for the following publication:**

| | |
|---|---|
| Title | Transfer Learning for Finetuning Large Language Models |
| Link to Publication, DOI | https://openreview.net/forum?id=gDeW6B8WCh<br>https://arxiv.org/abs/2411.01195 |
| Authors | Tobias Strangmann, Lennart Purucker, Jörg K.H. Franke, Ivo Rapant, Fabio Ferreira, Frank Hutter |
| Publication Status | Submitted to NeurIPS 2024 Workshop on Adaptive Foundation Models |
| Publisher, Date | - |
| Peer-Review-Process | yes |
| Rank | not ranked by CORE2023 (workshop) |

**Paper Summary**

This paper presents a new approach to finetuning large language models (LLMs) using transfer learning. The paper focuses on transferring knowledge about previous configurations from related finetuning tasks to new tasks. The authors introduce an adapted version of the Quick-Tune algorithm [1], originally developed for image classification tasks, and apply it as a meta-learner for the finetuning of LLMs. Central to this approach is a meta-dataset consisting of 1,800 finetuning runs of Microsoft's Phi-3 model on a board set of different hyperparameter configurations and using two optimizers, AdamW and the recently proposed AdamCPR [2]. The meta-dataset is used to optimize Quick-Tune as the meta-learner. This optimization enables the transfer of knowledge from previously optimized tasks to new ones, allowing for more efficient and effective finetuning across different domains.

The experiments, conducted on eight synthetic question-answer datasets, demonstrate that the adapted Quick-Tune method outperforms default finetuning approaches and other optimization baselines in terms of accuracy and efficiency. Empirical results further reveal that not refitting the performance and cost surrogate models leads to better generalization and performance across tasks, with the authors hypothesizing that avoiding task-specific refitting enhances overall transferability. The key contributions of the paper are:

1. Introduction of *Quick-Tune* as a meta-learner to transfer knowledge from related tasks for finetuning large language models (LLMs).
2. Creation of a meta-dataset consisting of 1,800 finetuning runs of Microsoft's Phi-3 model to optimize the meta-learner and improve generalization across tasks.
3. Experimental results demonstrate that the adapted *Quick-Tune* approach outperforms default finetuning methods and other optimization baselines across eight synthetic question-answer datasets.

[1] Arango, S. P., Ferreira, F., Kadra, A., Hutter, F., & Grabocka, J. (2024). *Quick-Tune: Quickly Learning Which Pretrained Model to Finetune and How*. In The Twelfth International Conference on Learning Representations (ICLR 2024). Paper: https://openreview.net/forum?id=tqh1zdXIra

[2] Franke J.K.H., Hefenbrock, M., Koehler, G., & Hutter, F. (2024). Improving Deep Learning Optimization through Constrained Parameter Regularization. In The Thirty-Eighth Annual Conference on Neural Information Processing Systems (NeurIPS 2024). Paper: https://arxiv.org/abs/2311.09058

**Contributions Listing**

| **Name** | **Contributions** | **Signature** |
|---|---|---|
| Tobias Strangmann | Owned and led the development of the adaptation of *Quick-Tune* to LLMs and handled all core implementations;<br><br>Owned, led, and implemented all experiments conducted;<br><br>Owned and led the writing of the paper, as well as reviewing and rebutting it. | Signiert von:<br>T. Strangmann<br>3E26F39BF9D74A6...<br>05.11.2024 |
| Lennart Purucker | Co-supervised the project alongside Jörg and Fabio;<br><br>Contributed to writing and reviewing the paper and identifying key research questions;<br><br>Framed the research and experiments with a topic-wise focus on hyperparameter optimization (HPO), finetuning, and transfer learning.<br><br>Contributed to shaping the project's vision and methodology in collaboration with the supervisory team;<br><br>Provided input on shaping the vision of the project. | Signiert von:<br>Lennart Oswald Purucker<br>6A52A22B8876416...<br>05.11.2024 |

Docusign Envelope ID: 5105FC86-E829-4EE8-A6B6-9CAA69FF6C4B

| | | |
|---|---|---|
| Jörg K.H. Franke | Proposed the project vision for more efficient LLM finetuning by transfer learning ;<br><br>Supervised Tobias throughout the project;<br><br>Designed the synthetic data generation and experiments for LLM tuning;<br><br>Contributed to framing the paper with a focus on LLM tuning and how to adapt Quick-Tune for LLMs; | Signed by:<br>DC6598DF2302491...<br>05/11/2024 |
| Ivo Rapant | Acted as the Quick-Tune code expert and supported Tobias with coding-related questions;<br><br>Ran additonal experiments involving Quick-Tune; | Signed by:<br>E18D86EC0C94416...<br>11/6/2024 |
| Fabio Ferreira | Co-supervised the project alongside Jörg and Lennart;<br><br>Contributed to framing the paper and supported with Quick-Tune-related questions;<br><br>Contributed to writing the paper and reviewing, as well as identifying key research questions;<br><br>Provided input on shaping the vision of the project. | DocuSigned by:<br>CA7363FD31BF45C...<br>05.11.2024 |
| Frank Hutter | Proposed Quick-Tune's adaptation to other domains; and overall contributed to shaping the project's vision and methodology;<br><br>Helped conceptualize the problem;<br><br>Supported in reviewing, and editing the paper;<br><br>Supervised Lennart, Jörg, and Fabio. | Signed by:<br>3CDF1E88127C47F...<br>06/11/2024 |
