# Supplementary material for: Meta-Learning and Synthetic Data for Automated Pretraining and Finetuning
Source: arXiv:2506.12161 source file (2025-06-11)
Supplement: Supplementary file 8 [file 2024_quicktune_soc.pdf]

Docusign Envelope ID: B02E5822-9347-4BCE-B021-C519F6647009

**Statement of Contributions for the following publication:**

| | |
|---|---|
| Title | Quick-Tune: Quickly Learning Which Pretrained Model to Finetune and How |
| Link to Publication, DOI | https://openreview.net/forum?id=tqh1zdXIra |
| Authors | Sebastian Pineda Arango, Fabio Ferreira, Arlind Kadra, Frank Hutter and Josif Grabocka |
| Publication Status | Accepted and published |
| Publisher, Date | The Twelfth International Conference on Learning Representations (ICLR), 2024 |
| Peer-Review-Process | Yes |
| Rank | Ranked A* by the CORE2023 ranking |

**Paper Summary**

This paper introduces QuickTune, a method to select a model and its hyperparameters (a.k.a. pipelines) for finetuning efficiently. To this end, this work applies in a novel way multifidelity, cost-awareness, and meta-learning. It contains the following contributions:

1. We present an effective methodology for quickly selecting models from hubs and jointly tuning their hyperparameters.
2. We design an extensive search space that covers common finetuning strategies. In this space, we train and evaluate 20k models and dataset combinations to arrive at a large meta-dataset to meta-learn a gray-box performance predictor and benchmark our approach.
3. We compare against multiple baselines, such as common finetuning strategies and state-of-the-art HPO methods, and show the efficacy of our approach by outperforming all of the competitor baselines.

Docusign Envelope ID: B02E5822-9347-4BCE-B021-C519F6647009

**Contributions Listing**

| **Name** | **Contributions** | **Signature and Date** |
|---|---|---|
| Sebastian Pineda Arango | Co-led the conceptualization of the idea;<br><br>Owned and was responsible for implementing the proposed method.<br><br>Created the repository with the final version of the code.<br><br>Had a key role in data curation of Meta-album datasets (together with Fabio) and loading, integrating finetuning strategies such as Co-tuning, Stoch-norm, SP-Regularization, Layer freezing (together with Fabio), and others. Defined the search space and config space (together with Fabio and Arlind). Integrated the architectures to finetune (together with Fabio). Generated the meta-dataset. Performed failure analysis (together with Arlind).<br><br>Created the initial draft of all sections. Co-led writing the majority of the paper including contributions to all parts of the paper. Created the visualizations of the final paper version. Contributed significantly to the rebuttal process (together with Arlind). | DocuSigned by:<br>Sebastian Pineda Arango<br>FC1C0379C4234BB...<br>7/1/2024 |

Docusign Envelope ID: B02E5822-9347-4BCE-B021-C519F6647009

| | | |
|---|---|---|
| Fabio Ferreira | Co-led the conceptualization of the idea;<br><br>Owned and was responsible for implementing the execution pipeline for creating the meta-dataset on the cluster infrastructure and provided initial templates for running pipelines on the cluster.<br><br>Had a key role in data curation (together with Sebastian), config space definition (together with Sebastian and Arlind), coding for the DINO experiments (section “Hypothesis 4”), implementing architectures and developing finetuning strategies (both together with Sebastian).<br>Co-led writing the paper including contributions to all parts of the paper but the parts of the paper he had the major contributions were:<br>The Related Work (together with Josif and Frank), Quick-Tune Meta-Dataset (together with Sebastian), Experiments “Hypothesis 4”, he also helped with the vision and introduction of the paper. | DocuSigned by:<br>CA7363FD31BF45C...<br>7/10/2024 |
| Arlind Kadra | Co-led the conceptualization of the idea;<br><br>Owned and was responsible for the HPO baseline experiments (section “Hypothesis 2”), including code development and experiment execution (together with Sebastian). Helped with the config space definition (together with Sebastian and Fabio); Provided the code for the core component of the proposed method (DyHPO algorithm). Performed failure analysis (together with Sebastian).<br><br>Co-led writing the paper including contributions to all parts of the paper but the parts of the paper he had the major contributions were:<br>Experiments and Supplementary sections;<br><br>Contributed to the rebuttal process (together with Sebastian). | DocuSigned by:<br>655FFB067F26476...<br>7/4/2024 |

Docusign Envelope ID: B02E5822-9347-4BCE-B021-C519F6647009

| | | |
|---|---|---|
| Frank Hutter | Helped with reviewing and editing the paper;<br><br>Helped conceptualize the problem;<br><br>Co-led supervision of the project. | Signed by:<br>3CDF1E88127C47F...<br>7/10/2024 |
| Josif Grabocka | Co-led writing the paper including contributions to all parts of the paper but the parts of the paper he had the major contributions were:<br>Introduction and Method;<br><br>Helped with reviewing and editing the paper;<br><br>Helped conceptualize the problem;<br><br>Co-led supervision of the project. | Signed by:<br>Josif Grabocka<br>257E43784D71473...<br>7/10/2024<br><br>Signed by:<br>Josif Grabocka<br>257E43784D71473... |
